# Supplementary material for: APEX: Assumption-free Projection-based Embedding eXamination Metric for Generative Distribution Evaluation
Source: arXiv:2605.07786 source file (2026-10-09)
Supplement: Supplementary file 1 [file appendix_intra_dataset.tex]

\section{Intra-dataset stability} \label{sec:app_intradataset}
In this section, we extend the results on intra-dataset stability giving the score each metric achieves on every dataset. 
We precise that KID and DINO+MMD should be interpreted cautiously, since their finite-sample biases are close to zero, making CV poorly conditioned. \cate{add FWD?}
\begin{longtable}{llccc}
\caption{\textbf{Intra-dataset real-vs-real statistics.}
For each dataset and metric, we report the finite-sample bias $\bar{\nu}$, the standard deviation $\sigma$, and the coefficient of variation $\mathrm{CV}=\sigma/|\bar{\nu}|$ over $R{=}20$ random splits.}
\label{tab:intradataset-full} \\
\toprule
Dataset & Metric & $\bar{\nu}$ & $\sigma$ & CV \\
\midrule
\endfirsthead

\toprule
Dataset & Metric & $\bar{\nu}$ & $\sigma$ & CV \\
\midrule
\endhead

\midrule
\multicolumn{5}{r}{\emph{continued on next page}} \\
\endfoot

\bottomrule
\multicolumn{5}{p{0.9\linewidth}}{\footnotesize $^\dagger$CV is poorly conditioned when the mean real-vs-real distance is close to zero.} \\
\endlastfoot

\multirow{6}{*}{CelebA-HQ}
& FID
& $5.73$ & $5.64{\times}10^{-2}$ & ${0.0098}$ \\
& KID$^\dagger$
& $-7.28{\times}10^{-6}$ & $2.35{\times}10^{-5}$ & $3.23$ \\
& CMMD
& $2.99{\times}10^{-1}$ & $3.08{\times}10^{-2}$ & $0.1029$ \\
& DINO+MMD$^\dagger$
& $4.34{\times}10^{-6}$ & $3.33{\times}10^{-5}$ & $7.68$ \\
\rowcolor{gray!10}
& \ours-CLIP
& $1.54{\times}10^{-2}$ & $4.78{\times}10^{-4}$ & ${{0.0310}}$ \\
\rowcolor{gray!10}
& \ours-DINO
& $5.32{\times}10^{-4}$ & $3.12{\times}10^{-5}$ & ${0.0587}$ \\

\midrule
\multirow{6}{*}{ChestX-ray}
& FID
& $3.84$ & $2.52{\times}10^{-2}$ & ${0.0065}$ \\
& KID$^\dagger$
& $-1.34{\times}10^{-5}$ & $1.83{\times}10^{-5}$ & $1.36$ \\
& CMMD
& $7.10{\times}10^{-2}$ & $2.00{\times}10^{-2}$ & $0.2823$ \\
& DINO+MMD$^\dagger$
& $-4.83{\times}10^{-6}$ & $2.42{\times}10^{-5}$ & $5.01$ \\
\rowcolor{gray!10}
& \ours-CLIP
& $6.61{\times}10^{-3}$ & $3.19{\times}10^{-4}$ & ${0.0483}$ \\
\rowcolor{gray!10}
& \ours-DINO
& $1.44{\times}10^{-4}$ & $6.70{\times}10^{-6}$ & ${{0.0465}}$ \\

\midrule
\multirow{6}{*}{COCO-30k}
& FID
& $13.14$ & $8.89{\times}10^{-2}$ & ${0.0068}$ \\
& KID$^\dagger$
& $1.12{\times}10^{-5}$ & $4.11{\times}10^{-5}$ & $3.67$ \\
& CMMD
& $3.22{\times}10^{-1}$ & $1.98{\times}10^{-2}$ & $0.0615$ \\
& DINO+MMD$^\dagger$
& $1.83{\times}10^{-6}$ & $9.66{\times}10^{-6}$ & $5.28$ \\
\rowcolor{gray!10}
& \ours-CLIP
& $1.67{\times}10^{-2}$ & $3.83{\times}10^{-4}$ & ${{0.0230}}$ \\
\rowcolor{gray!10}
& \ours-DINO
& $6.38{\times}10^{-4}$ & $1.48{\times}10^{-5}$ & ${0.0233}$ \\

\midrule
\multirow{6}{*}{HAM10000}
& FID
& $5.79$ & $6.79{\times}10^{-2}$ & ${0.0117}$ \\
& KID$^\dagger$
& $7.47{\times}10^{-6}$ & $4.57{\times}10^{-5}$ & $6.11$ \\
& CMMD
& $1.78{\times}10^{-1}$ & $4.66{\times}10^{-2}$ & $0.2620$ \\
& DINO+MMD$^\dagger$
& $4.46{\times}10^{-6}$ & $2.42{\times}10^{-5}$ & $5.43$ \\
\rowcolor{gray!10}
& \ours-CLIP
& $9.74{\times}10^{-3}$ & $5.98{\times}10^{-4}$ & ${0.0614}$ \\
\rowcolor{gray!10}
& \ours-DINO
& $4.14{\times}10^{-4}$ & $2.06{\times}10^{-5}$ & ${{0.0497}}$ \\

\midrule
\multirow{6}{*}{RESISC45}
& FID
& $10.64$ & $8.95{\times}10^{-2}$ & ${0.0084}$ \\
& KID$^\dagger$
& $1.02{\times}10^{-5}$ & $3.84{\times}10^{-5}$ & $3.75$ \\
& CMMD
& $2.31{\times}10^{-1}$ & $3.74{\times}10^{-2}$ & $0.1621$ \\
& DINO+MMD$^\dagger$
& $1.90{\times}10^{-6}$ & $1.82{\times}10^{-5}$ & $9.56$ \\
\rowcolor{gray!10}
& \ours-CLIP
& $1.23{\times}10^{-2}$ & $5.10{\times}10^{-4}$ & ${0.0414}$ \\
\rowcolor{gray!10}
& \ours-DINO
& $5.44{\times}10^{-4}$ & $2.06{\times}10^{-5}$ & ${{0.0378}}$ \\

\end{longtable}
